# Supplementary material for: DRaCoN -- Differentiable Rasterization Conditioned Neural Radiance Fields for Articulated Avatars
Source: arXiv:2203.15798 source file (2022-03-29)
Supplement: Supplementary file 1 [file Supplm.tex]

\documentclass[10pt,twocolumn,letterpaper]{article}

% Include other packages here, before hyperref.
\usepackage{graphicx}
\usepackage{amsmath}
\usepackage{amssymb}
\usepackage{booktabs}
\usepackage{xcolor}
\usepackage{comment}
\usepackage[pagebackref,breaklinks,colorlinks]{hyperref}
\usepackage[accsupp]{axessibility}
\usepackage{cvpr}              % To produce the CAMERA-READY version

% If you comment hyperref and then uncomment it, you should delete
% egpaper.aux before re-running latex.  (Or just hit 'q' on the first latex
% run, let it finish, and you should be clear).
% \usepackage[pagebackref,breaklinks,colorlinks,bookmarks=false]{hyperref}
% \usepackage[table]{xcolor}
\usepackage{ruler}
% \usepackage[width=122mm,left=12mm,paperwidth=146mm,height=193mm,top=12mm,paperheight=217mm]{geometry} 

% Support for easy cross-referencing
\usepackage[capitalize]{cleveref}
\crefname{section}{Sec.}{Secs.}
\Crefname{section}{Section}{Sections}
\Crefname{table}{Table}{Tables}
\crefname{table}{Tab.}{Tabs.}

% If you wish to avoid re-using figure, table, and equation numbers from
% the main paper, please uncomment the following and change the numbers
% appropriately.
%\setcounter{figure}{2}
%\setcounter{table}{1}
%\setcounter{equation}{2}

% If you wish to avoid re-using reference numbers from the main paper,
% please uncomment the following and change the counter for `enumiv' to
% the number of references you have in the main paper (here, 6).
%\let\oldthebibliography=\thebibliography
%\let\oldendthebibliography=\endthebibliography
%\renewenvironment{thebibliography}[1]{%
%     \oldthebibliography{#1}%
%     \setcounter{enumiv}{6}%
%}{\oldendthebibliography}

%%%%%%%%% PAPER ID  - PLEASE UPDATE
% \def\cvprPaperID{7062} % *** Enter the CVPR Paper ID here
% \def\confName{CVPR}
% \def\confYear{2022}

% \begin{document}
\begin{document}
% \renewcommand\thelinenumber{\color[rgb]{0.2,0.5,0.8}\normalfont\sffamily\scriptsize\arabic{linenumber}\color[rgb]{0,0,0}}
% \renewcommand\makeLineNumber {\hss\thelinenumber\ \hspace{6mm} \rlap{\hskip\textwidth\ \hspace{6.5mm}\thelinenumber}}
% \linenumbers
\pagestyle{headings}
\mainmatter
\def\ECCVSubNumber{5732}  % Insert your submission number here

\title{DRaCoN -- Supplementary Materials}
% \title{MINA: Multi-Identity Neural Avatar \\ Learning via Differentiable Rasterization Conditioned NeRF}

% INITIAL SUBMISSION 
%\begin{comment}
\titlerunning{DRaCoN -- ECCV-22 submission ID \ECCVSubNumber} 
\authorrunning{DRaCoN -- ECCV-22 submission ID \ECCVSubNumber} 
\author{Anonymous ECCV submission}
\institute{Paper ID \ECCVSubNumber}
%\end{comment}
%******************

% CAMERA READY SUBMISSION
\begin{comment}
\titlerunning{Abbreviated paper title}
\end{comment}
%%%%%%%%% TITLE - PLEASE UPDATE
% \title{DRaCoN - Supplementary Materials}  % **** Enter the paper title here

\maketitle
\thispagestyle{empty}
\appendix

%%%%%%%%% BODY TEXT - ENTER YOUR RESPONSE BELOW
\section{Network details}
Fig.~\ref{fig:sup-anr} and Fig.~\ref{fig:sup-adanerf} show the architecture of the generator used in the \emph{DiffRas} module and the \emph{Ada-NeRF} generator respectively. We use a U-Net architecture for the generator in the \emph{DiffRas} module to texture the UV image.

\section{Training details}
We train models on both H3.6M and ZJU-Mocap on 300 frames for each identity. We train our models for 160k iterations which takes around 16 hours on 2 NVIDIA A40 GPUs. All models are trained with a learning rate of $5e-4$. The neural texture has a spatial resolution of $64 \times 64$ with $64$ channels.

\section{Renderer specifics}
Our Differentiable Rasterization based generator is defined as follows. For a mesh $\mathbf{M}=(\mathbf{V},\mathbf{F})$, we define a rasterization function $\Psi:(|\mathbf{V}| \times |\mathbf{F}| \times \mathbb{R}^{3 \times 3} ) \rightarrow \mathbb{R}^{H \times W \times 2}$ such that:
\begin{equation}
    \mathbf{I}^{uv} = \Psi(\mathbf{V},\mathbf{F},\mathbf{\Pi})
\end{equation}
Where $\mathbf{I}^{uv}$ is an image where each pixel represents the uv-coordinates of the point on the mesh visible from the given camera viewpoint and $\mathbf{\Pi}$ is the world-to-camera projection matrix.

The UV image is then used to sample the identity specific neural texture $\mathbf{Z} \in \mathbb{R}^{S \times S \times D}$ using a bilinear sampling operator $\Phi$
\begin{equation}
    \mathbf{I}^{nt} = \Phi(\mathbf{I}^{uv},\mathbf{Z})
\end{equation}
where $\mathbf{I}^{nt} \in \mathbb{R}^{H \times W \times D}$

The spatial extent of the rendered mesh in $\mathbf{I}^{nt}$ is limited to the shape captured by the parametric SMPL model and does not capture clothing and identity specific shape information.  We then use a Pix2pix style generator network~\cite{isola2017image} $\mathcal{N}_{feat}$ to account for identity and pose specific geometric deformation.
\begin{equation}
    \mathbf{I}^{feat} = \mathcal{N}_{feat}(\mathbf{I}^{nt})
\end{equation}
\begin{equation}
    \texttt{DiffRas} = \mathcal{N}_{feat} \circ \Phi \circ \Psi
\end{equation}

Given the above $\mathbf{I}^{feat}$, for any spatial location $\mathbf{x}$ in posed space we obtain the corresponding  pixel location $x = \mathbf{\Pi} \mathbf{x}$ and obtain the pixel aligned feature as:
\begin{equation}
    f_{\mathbf{x}} = \Phi(x, \mathbf{I}^{feat})
    \label{eq:fx}
\end{equation}

\section{Affine Transform calculaiton}
For every image $\mathbf{I}_i$ corresponding to frame $i$, we calculate the tightest bounding box $\mathbf{B}_i \in \mathbb{R}^{2 \times 2 \times 2 \times 2}$ around the actor, where 
\begin{equation*}
    \mathbf{B} = [(x_i^{(1)},y_i^{(1)}),(x_i^{(2)},y_i^{(2)}),(x_i^{(3)},y_i^{(3)}),(x_i^{(4)},y_i^{(4)})] 
\end{equation*}
represents the four corners of the bounding box. We then update the corners such that the height and width of the updated bounding box $\tilde{\mathbf{B}}$ are equal. Let $\texttt{Cr}(\mathbf{I},\mathbf{B})$ represent image $\mathbf{I}$ cropped to bounding box $\mathbf{B}$. We calculate affine transformation $\mathbf{\Omega}_i$ such that  $\texttt{Cr}(\mathbf{I},\mathbf{B})$ is transformed into a $256 \times 256$ image before feeding it into the generator of the \emph{DiffRas} module. This ensures that the generator always sees similarly sized inputs of actors in posed space.
The projection of any spatial location $\mathbf{x}$ inside the bounding box is then obtained as follows:
%pixel aligned features for frame $i$ for any world space point $\mathbf{x}$ are then obtained as follows:
\begin{equation}
x = \mathbf{\Omega}_i \mathbf{\Pi}_i \mathbf{x}.
\end{equation}
The pixel aligned feature $f_\mathbf{x}$ can then be obtained as in Equation.~\ref{eq:fx}

\section{User study}
Since most of the metrics used serve mostly as a proxy to perceptual quality, we perform a user study to compare avatars generated using different methods. Particularly, each user is presented with 20 randomly sampled views in novel poses across 4 different identities for 8 seconds. The user is asked to rate which of the 4 avatars looks most realistic. We collected this data over 26 random subjects. The demographics include both technical experts who work on digital avatars and general audience. The results (Table. ~\ref{tab:user}) of the study indicate that our method is preferred $\textbf{74 \%}$ of the time as compared to the the next highest rated method (Neuralbody \cite{peng2021neural}) at $19 \%$

\section{Ablation study}
Figure. ~\ref{fig:3dm} shows the difference in predicted geometry with different losses removed. Particularly, we see that the eikonal regularizer helps extract a closed mesh surface from the SDF network. The TV loss encourages the extracted surface to be smooth and the face loss improves the structure around the face in the learnt geometry. 
\begin{figure}
    \centering
    \includegraphics[trim={0 0.5cm 0 0}, width=1.0\linewidth]{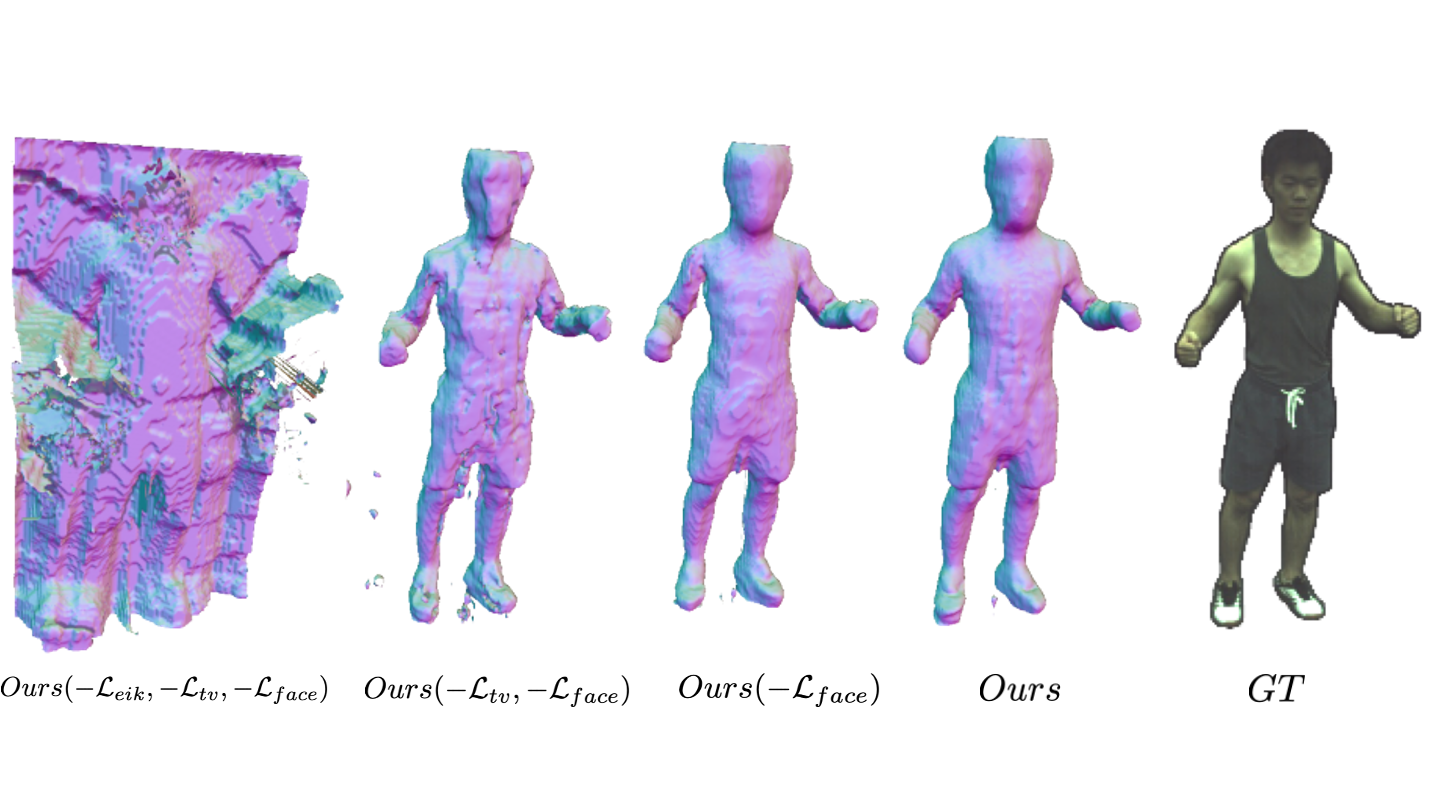}
    \caption{Ablation study on predicted geometry with different losses removed. We see that the eikonal loss is necessary to learn a meaningful geometry. The 3D tv-loss ensures smoothness and the face loss adds some additional structure around the face.}
    \label{fig:3dm}
\end{figure}
\begin{figure*}
    \centering
    \includegraphics[ width=1.0\linewidth]{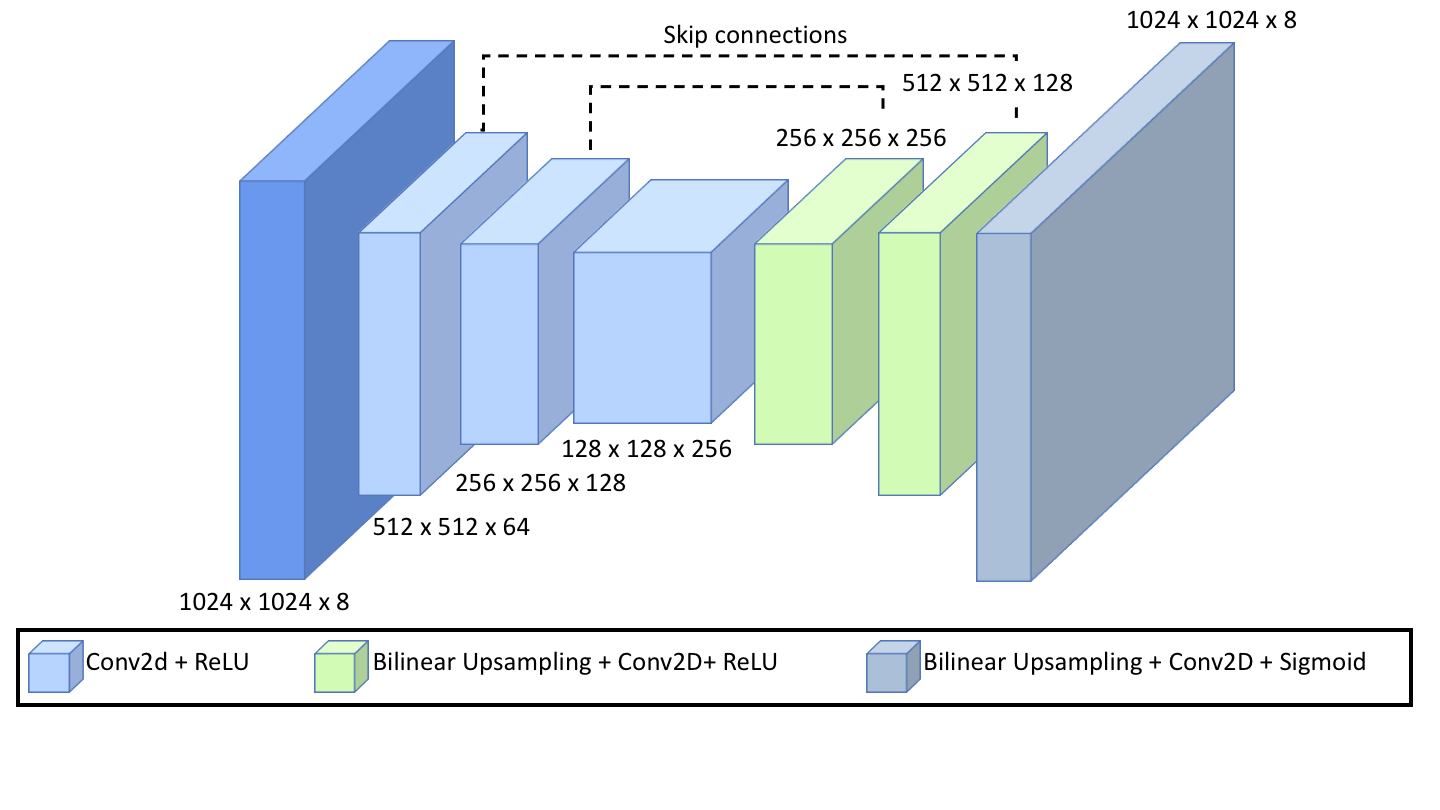}
    \caption{Architecture of the Generator in the DiffRas Module}
    \label{fig:sup-anr}
\end{figure*}
\input{latex/figures/fig-sup-adanerf}
\begin{figure*}
    \centering
    \includegraphics[trim={0 0.5cm 0 0}, width=1.0\linewidth]{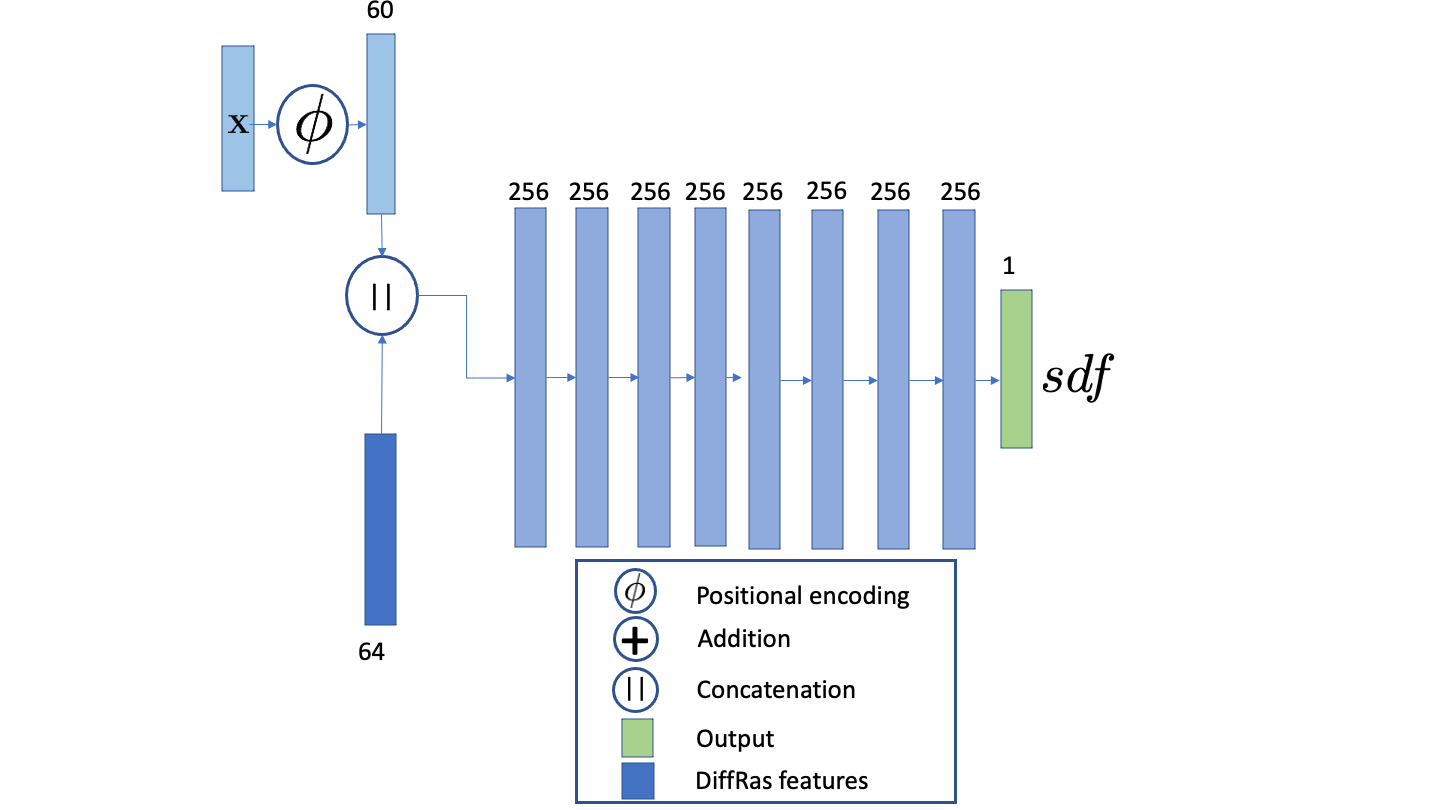}
    \caption{Architecture of the Generator in the SDF Module}
    \label{fig:sup-adanerf}
\end{figure*}
\begin{table*}[h]
\small
    \centering
    % \rowcolors{2}{gray!15}{white}
    \begin{tabular}{l | cc}
    \toprule
      & Num Votes & ~Mean Preference \\
    \specialrule{0.12em}{0.05em}{0.05em}
     A-Nerf~\cite{su2021anerf}  & $28$ & $5.00 \% \pm 0.14$ \\
     NeuralBody~\cite{peng2021neural} & $103$ & $19.50 \% \pm 3.8$ \\
     Anim-NeRF~\cite{peng2021animatable} & $12$ & $2.39 \% \pm 0.64$ \\
     \specialrule{0.08em}{0.05em}{0.05em}
     Ours & $377$ & $\textbf{72.5} \% \pm 4.6$ \\
    \bottomrule
    \end{tabular}
    \caption{User study performed on novel poses over 4 different ZJU identities.}
    % \vspace{-5mm}
    \label{tab:user}
\end{table*}
\begin{table*}[h]
\small
    \centering
    % \rowcolors{2}{gray!15}{white}
    \begin{tabular}{c ccc | ccc | ccc}
    \toprule
     &\multicolumn{3}{c}{Neuralbody} &\multicolumn{3}{c}{Animatable NeRF} & \multicolumn{3}{c}{Ours} \\
       & SSIM $\uparrow$ & PSNR $\uparrow$ & LPIPS $\downarrow$ & SSIM $\uparrow$ & PSNR $\uparrow$ & LPIPS $\downarrow$ & SSIM $\uparrow$ & PSNR $\uparrow$ & LPIPS $\downarrow$ \\
     \specialrule{0.12em}{0.05em}{0.05em}
    S1 & $0.821$ & $20.925$ & $0.025$ & $0.841$ & $18.491$ & $0.027$ & $\textbf{0.852}$ & $\textbf{22.720}$ & $0.013$ \\
    S5 & $0.835$ & $24.183$ & $0.017$ & $0.865$ & $21.071$ & $0.022$ & $\textbf{0.883}$ & $\textbf{25.307}$ & $0.009$ \\
    S6 & $0.816$ & $21.608$ & $0.023$ & $0.834$ & $20.315$ & $0.028$ & $\textbf{0.856}$ & $\textbf{21.399}$ & $0.014$ \\
    S7 & $\textbf{0.847}$ & $\textbf{22.267}$ & $0.018$ & $0.838$ & $21.612$ & $0.023$ & $0.835$ & $22.256$ & $0.013$ \\ 
    S8 & $0.822$ & $20.214$ & $0.025$ & $0.852$ & $21.582$ & $0.024$ & $\textbf{0.890}$ & $\textbf{23.949}$ & $0.013$ \\
    S9 & $0.853$ & $21.773$ & $0.026$ & $0.872$ & $22.394$ & $0.031$ & $\textbf{0.885}$ & $\textbf{25.855}$ & $0.017$ \\
    S11 & $0.857$ & $21.885$ & $0.029$ & $0.879$ & $23.131$ & $0.028$ & $\textbf{0.888}$ & $\textbf{25.951}$ & $0.017$ \\
    \bottomrule
    \end{tabular}
    \caption{Novel view synthesis results on Human3.6M.}
    \label{tab:comparison}
\end{table*}

% \section{Limitations}
% Fig.~\ref{fig:sup-fail} demonstrates the limitation of our approach. Particularly for constricted poses where multiple joints are close to each other, the warping module fails to identify the appropriate blend weights to canonicalize the points from posed space. This error propagates to the rendering stage since the radiance calculation is affected by inaccurate canonicalization.
% \input{latex/figures/fig-sup-failure}

\section{H3.6M additional comparisons}
Table.~\ref{tab:comparison} provides comparison of our approach against Neuralbody\cite{peng2021neural} and Animatable-Nerf \cite{peng2021animatable} evaluated over 30 novel poses. 

% The accompanying video additionally provides pose retargetting onto avatars learned using our multi-identity model trained over 5 identities.

% \section{Comparison against multi-ID Neuralbody}

% \section{Additional results}

% \section{C-NeRF vs AdaNeRF}
% \begin{table}[h]
% \small
%     \centering
%     \begin{tabular}{c|ccccc}
    
%      & MSE  $\downarrow$ & SSIM $\uparrow$ & PSNR $\uparrow$ & \multicolumn{2}{c}{LPIPS $\downarrow$} \\
%      &&&& Alexnet & VGG \\
%      \specialrule{0.12em}{0.05em}{0.05em}
%     D-NeRF  & $2.34$ & $0.946$ & $26.47$	& $0.082$ &	$0.058$ \\\
%     NHR     & $0.82$ &	$0.976$ & $30.98$ & $0.026$ & $0.024$ \\
%     NB & $0.66$ & $0.977$ & $31.93$ & $0.039$ &	$0.029$ \\
%     Anim-NeRF & $0.50$ &	$0.979$ &	$33.11$ &	$0.035$ &	$0.028$ \\ 
%     \hline
%     Ours & $\mathbf{0.32}$	& $\mathbf{0.985}$ & $\mathbf{35.22}$ & $\mathbf{0.023}$ & $\mathbf{0.022}$
%     \end{tabular}
%     \caption{Novel view synthesis results on Human3.6M dataset. Our approach outperforms recent baselines on most supervised metrics}
%     \vspace{-5mm}
%     \label{tab:comparison}
% \end{table}

%%%%%%%%% REFERENCES
{\small
\bibliographystyle{splncs04}
\bibliography{egbib}
}

\end{document}
